# Supplementary material for: Simultaneous observation of anti-damping and inverse spin Hall effect in La$_{0.67}$Sr$_{0.33}$MnO$_{3}$/Pt bilayer system
Source: arXiv:2005.07848 source file (2020-09-10)
Supplement: Supplementary file 1 [file bedanta_supplimentary.pdf]

# Simultaneous observation of anti-damping and inverse spin Hall effect in $La_{0.67}Sr_{0.33}MnO_3$/Pt bilayer system

Pushpendra Gupta[1], Braj Bhusan Singh[1], Koustuv Roy[1], Anirban Sarkar[2], Markus Waschk[2], Thomas Brueckel[2], and Subhankar Bedanta[1,*]

[1]Laboratory for Nanomagnetism and Magnetic Materials (LNMM), School of Physical Sciences, National Institute of Science Education and Research (NISER), HBNI, P.O.- Bhimpur Padanpur, Via - Jatni, 752050, India

[2]Forschungszentrum Jülich GmbH, Jülich Centre for Neutron Science (JCNS-2) and Peter Grünberg Institut (PGI-4), JARA-FIT, 52425 Jülich, Germany

Figure S1 shows the X-ray diffraction peaks of the sample S1. All diffraction peaks are corresponding to (001) plane of LSMO. Since LSMO and $SrTiO_3$ (STO) peaks lies on the similar diffraction angle due to well-matched lattice parameters, it is difficult to differentiate them from the x-ray diffraction pattern. We did not observe any other diffraction peaks corresponding to different orientation of planes. Therefore, we concluded that our LSMO thin films are epitaxial grown perpendicular to (001) plane of STO substrate.

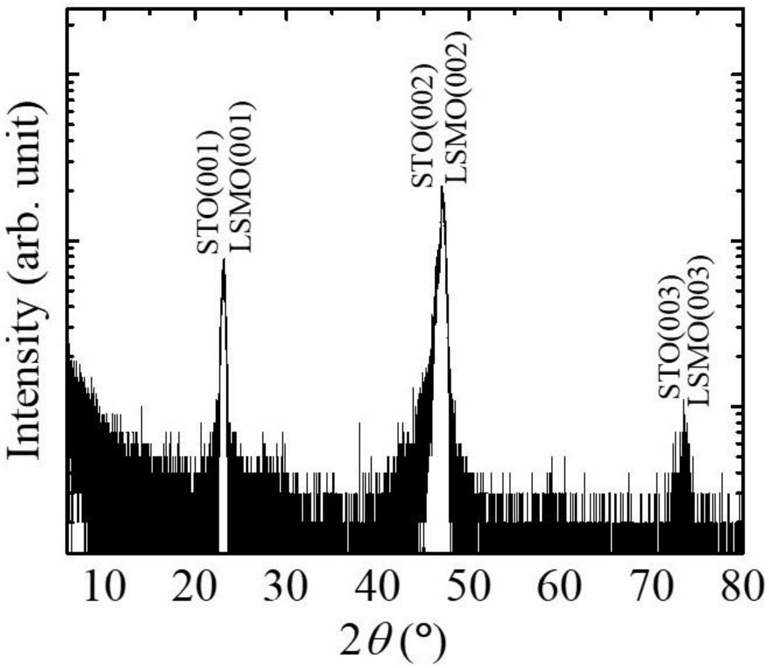


Fig. S1. X-ray diffraction pattern measured in $\theta$-$2\theta$ geometry of LSMO thin film (sample S1) deposited on STO (001) substrate by using oxygen plasma assisted molecular beam epitaxy (OMBE).

For comparison with standard sample to our results we have deposited one sample S4 with structure Si/$Co_{40}Fe_{40}B_{20}$ (5nm)/Pt (3nm) by DC sputtering. Figure S2 shows the ISHE data for the sample S4. We have separated $V_{sym}$ and $V_{asym}$ contribution from the data using equation (4). For

calculation of $\theta_{SHA}$ we have performed angle dependent ISHE measurements as shown in Figure S3. Value of $\theta_{SHA}$ for this sample calculated to 0.022 which match well with other previously reported values for Pt.

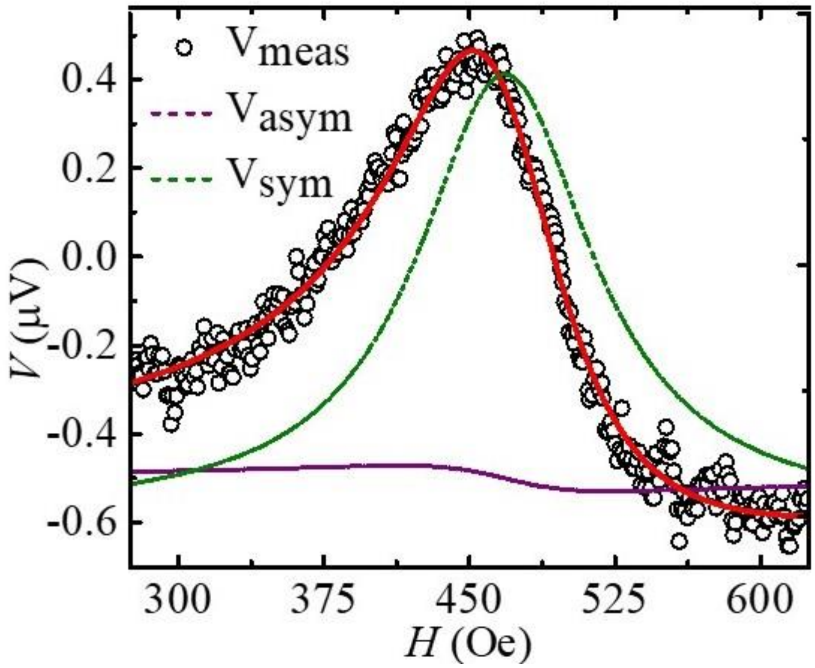


Fig. S2 ISHE voltage for samples Si/$Co_{40}Fe_{40}B_{20}$ (5nm)/Pt (3nm). Open circles (in blue) is the measured ISHE voltage and solid line (in red) represents the best fit of the data fitted by equation (4). Dash (in green) and dot (purple) lines represent the $V_{sym}$ and $V_{asym}$ components, respectively, evaluated by fitting to equation (4).

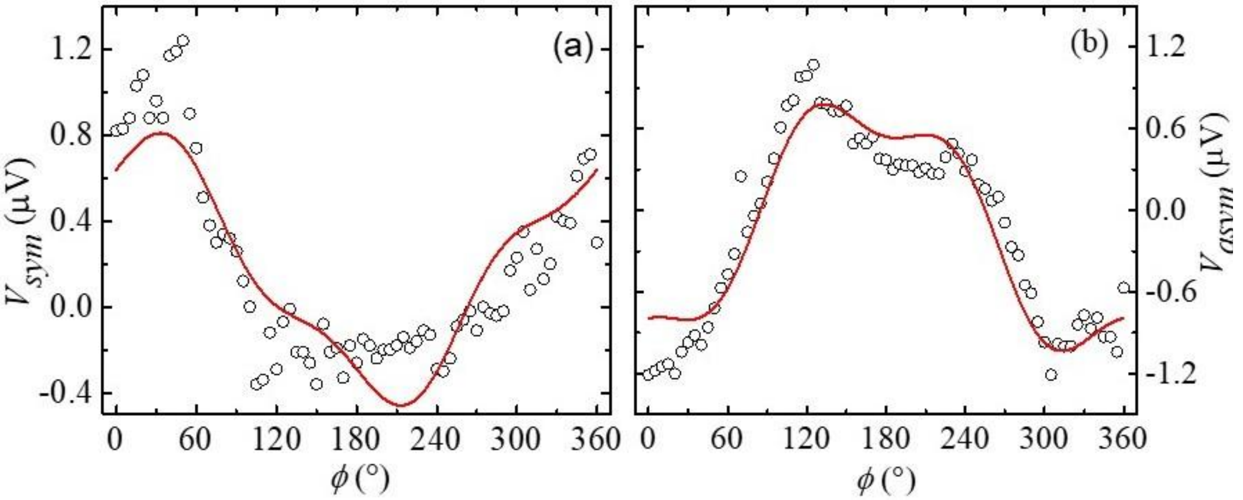


Fig. S3 (a) and (b) Angle dependent $V_{sym}$ and $V_{asym}$ for Si/$Co_{40}Fe_{40}B_{20}$ (5nm)/Pt (3nm) sample. Figure (a) and (b) were fitted by using equation (5) and equation (6) respectively.
